# Supplementary material for: Storage of photonic time-bin qubits for up to 20 ms in a rare-earth doped crystal
Source: arXiv:2109.06669 ancillary file (2022-03-23)
Supplement: Supplementary file 1 [file SM_Eu20msSpinStorage_final.pdf]

# Supplementary Information - Storage of photonic time-bin qubits for up to 20 ms in a rare-earth doped crystal

Antonio Ortu,[1] Adrian Holzäpfel,[1] Jean Etesse,[2] and Mikael Afzelius[1]

[1] *Département de Physique Appliquée, Université de Genève, Rue de l'Ecole-de-Médecine 20, 1205, Genève, Switzerland*
[2] *Université côte d'Azur, CNRS, Institut de Physique de Nice, Parc Valrose, Nice, Cedex 2, France*

(Dated: March 23, 2022)

### Supplementary Note 1: Crystals optical initialization

The preparation procedure begins with a class cleaning sequence[1]. This first step ensures that each frequency corresponds to a transition between the same two states for all atoms involved, for both the optical and RF transitions we are interested in. The frequencies of the cleaning pulses are the one corresponding to the $|g\rangle \leftrightarrow |e\rangle$ transition, on which the AFC is addressed, and four others with relative detuning of $-46$ MHz, $-6$ MHz, $+46$ MHz and $-92$ MHz, which correspond respectively to the spin transfer transition, the auxiliary transition for storing atoms not being part of the comb, and two additional transitions to empty states of other unwanted classes that might be addressed by the RF. The second step consists in polarizing the atomic population into the $|g\rangle = |\pm 5/2\rangle$ state, by optically pumping the other two ground states $|s\rangle = |\pm 3/2\rangle$ (the storage state) and $|a\rangle = |\pm 1/2\rangle$ (the auxiliary state). The third step involves the preparation of the AFC with optical pulses specifically modulated to have the corresponding comb-like spectrum[2], with defined maximum bandwidth $\Gamma$, teeth periodicity $\Delta$ and tooth width $\gamma$. A sequence of repumping pulses ensures that the $|s\rangle$ state stays empty in the process. All this steps are achieved by the memory preparation beam.

In parallel, via the filter preparation beam, the filtering crystals are initialized by a simpler optical pumping sequence which results in 2 MHz wide transparency and absorption windows, with central frequencies corresponding respectively to the $|g\rangle \rightarrow |e\rangle$ and $|s\rangle \rightarrow |e\rangle$ transitions. This way, ideally, only the photons emitted from the memory at the AFC transition will arrive at the detector, while the absorption profile blocks photons potentially emitted by atoms falling back along the $|e\rangle \rightarrow |s\rangle$ transition and possible scattered components of the final transfer pulse into the input spatial mode.

### Supplementary Note 2: Spin resonance

The inhomogeneous broadening of the $|g\rangle \leftrightarrow |s\rangle$ transition was characterized by probing the effect of spin dephasing on the retrieved signal in a modified spin storage sequence. A single input signal is stored in the memory and the amplitude of the retrieved signal is recorded while varying the temporal position $\tau$ of the second optical transfer pulse with respect to its position in the optimal rephasing case, while all other optical and RF pulses are kept fixed. The signal amplitude thus decreases as a function of $\tau$ according to a decay constant given by the inhomogenous broadening. The data is shown in Supplementary Figure 1, with a fit to the equation

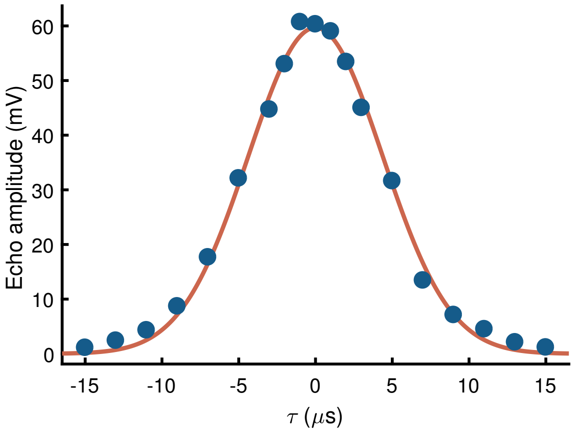


**Supplementary Figure 1: Spin resonance at 46 MHz.** Amplitude of retrieved signal after storage, as a function of the temporal shift $\tau$ applied to the center of the second transfer pulse with respect to its normal position for optimal dephasing. The solid line indicates the Gaussian fit used to extract the linewidth.

$$f(\tau) = a\, e^{-\frac{(\pi \Gamma_S \tau)^2}{2\ln(2)}}. \quad (1)$$

Here, the maximum amplitude $a$ and transition linewidth (FWHM) $\Gamma_s$ are free parameters. The resulting linewidth is $\Gamma_s = (61 \pm 2)$ kHz, with an error corresponding to a 95% confidence interval.

### Supplementary Note 3: RF sequence

All dynamical decoupling sequences were composed of adiabatic pulses with a hyperbolic secant amplitude profile[3] with a total duration (at the edges of which the signal is completely cut off) of 200 µs, a full width at half maximum of 50 µs and a frequency chirp of 300 kHz (about 5 times the spin broadening). The field shape is programmed via Matlab into an arbitrary wave generator and sent to a 100 W amplifier with 50 Ω impedance. This is coupled in output to a RF circulator and a custom

resonant circuit based on lumped elements. The circuit is needed to impedance-match the coil surrounding the crystal with the system generating the RF signal at 50 Ω. With this setup, we could achieve a Rabi frequency on the $|g\rangle \leftrightarrow |s\rangle$ transition of about 120 kHz, measured experimentally from the oscillation of population in the $|g\rangle$ state while driving the system at 46 MHz and optically probing on $|g\rangle \leftrightarrow |e\rangle$.

The optical transfer pulses on the optical transitions in the spin wave experiments are adiabatic HSH pulses[4], with flat central part of duration 10.7 µs, FWHM of the hyperbolic secant sides of 1.65 µs, total duration of 15 µs and frequency chirp of 1.5 MHz. The signal shape is programmed into an arbitrary wave generator with a central frequency of about 200 MHz, at the output of which the signal is amplified and fed to an acousto-optic modulator in double pass configuration.

The memory efficiency data points of the spin storage with bright pulses displayed in Figure 2 of the main text and used in the evaluation of the performance of the dynamical decoupling sequences are obtained from the time profile of the retrieved pulses by means of an oscilloscope. For each storage time and each DD sequence, the experiment is repeated 10 times. Each pulse profile is fitted with a Gaussian curve to extract the pulse area, which in turn is averaged over the 10 measurements, and divided by the area of a reference input pulse obtained analogously. The relative error (not shown in the figure) is dominated by shot-to-shot fluctuations and typically results in a standard deviation below 10 %. The inverse of the error of each data point is used as weight in the fitting procedure of the efficiency curve.

| DD type | $T_2^{\text{spin}}$ (ms) | $\eta_s(0)$ (%) | $m$ |
|---|---|---|---|
| XX | $70 \pm 2$ | $6.6 \pm 0.6$ | $2.4 \pm 0.4$ |
| XY-4 | $106 \pm 9$ | $7.7 \pm 1.6$ | $2.2 \pm 0.9$ |
| XY-8 | $154 \pm 11$ | $8.6 \pm 1.4$ | $1.5 \pm 0.3$ |
| XY-16 | $230 \pm 30$ | $6.4 \pm 1.7$ | $1.2 \pm 0.3$ |

**Supplementary Table 1: Dynamical decoupling with bright input pulses.** Fitted parameters of the spin storage curves with bright pulses for different DD sequences, according to equation 2. $T_2^{\text{spin}}$ = effective spin coherence time; $\eta_s(0)$ = extrapolated zero-time efficiency; $m$ = Mims factor.

Supplementary Table 1 reports all free parameters obtained from the least-squares fits of the spin storage efficiency curves as a function of storage time $T_s$. The model follows Mims' equation[5]

$$\eta_s(T_s) = \eta_s(0)\, e^{-2(T_s/T_2^{\text{spin}})^m}, \quad (2)$$

which takes into account the deviation from a pure exponential behavior due to spectral diffusion via the parameter $m$. Errors correspond to 95 % confidence intervals.

Supplementary Table 2 is an extension of Table 1 of the main text, displaying the average results of the storage experiments at the single photon level. The results are obtained from averaging the raw counts over the 6 time modes of duration $T_m = 1.65$ µs each. Errors are obtained from the standard deviation of a Poissonian distribution of the raw counts and propagated on the average considering the 6 modes as independent. The quantities $\mu_{\text{in}}$ and $p_N$ correspond to average number of photons at the memory output. They are obtained from the raw counts by dividing by the number of experiment repetitions, averaging over the 6 modes, and dividing by the detector efficiency $\eta_D = 57$ % and cryostat-to-detector path transmission (typically between 17 and 20 % depending on the specific experimental run). See also the Methods section of the main text.

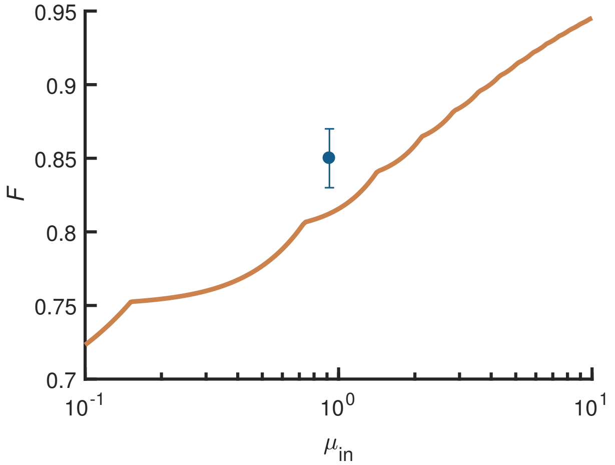


**Supplementary Figure 2: Classical limit of memory fidelity.** The solid line represents the classical memory fidelity $F$ achievable with a qubit mean photon number $\mu_{in}$, for a memory efficiency of 7.39%, according to the criterion by Specht et al.[6]. The data point represents the measured qubit fidelity measured at 20 ms, where the error bar represents ± one standard deviation.

Supplementary Table 3 reports the same quantities obtained separately in each temporal mode for the case $T_s = 20$ ms.

### Supplementary Note 4: Qubit tomography

Supplementary Table 4 displays additional details on the qubit storage. The raw counts in the interference temporal bins are used to calculate the visibility relative to each basis, from which a full tomography of the state can be derived. To increase the repetition rate of the experiment, two of the six temporal modes of the memory were used as for the interference of two different qubits respectively. The projection basis at readout is chosen by changing the relative phase $\theta$ of the two HSH components

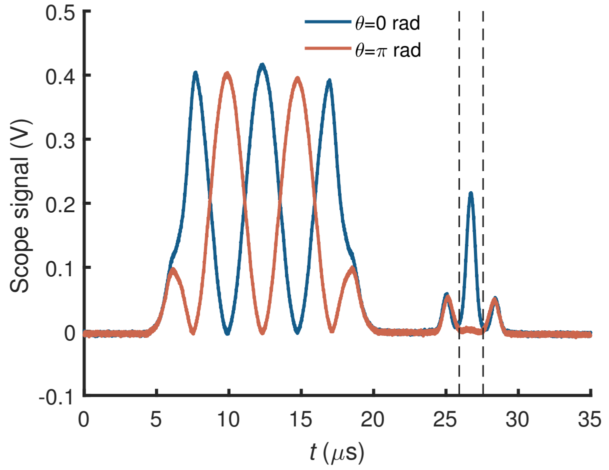


**Supplementary Figure 3: Analyzer readout with bright pulses.** Readout of a storage experiment of two bright input pulses in adjacent time modes, emulating a qubit experiment. The transmitted component of cHSH analyzer pulse and the retrieved modes are visible for two values of $\theta$ corresponding to orthogonal projections on the x basis of the qubit experiment. The dashed lines indicate the time bin from which the fidelity is measured.

of the cHSH pulse. For the trivial case of the z basis, the readout pulse is the same single HSH used in the other multimode spin-wave storage experiments, and the output signal is simply the retrieved qubit after storage on the same base as the input. In this particular case, the average visibility is calculated from the counts in modes 2 and 5 (the retrieved early components of the two stored qubits) and the counts in modes 3 and 6 (the retrieved late components).

The direct inversion method[7] results in a Bloch vector $\mathbf{r} = (V_{\mathrm{x}}, V_{\mathrm{y}}, V_{\mathrm{z}})$, where $V_j$ are the visibilities measured in directions $j = \mathrm{x}, \mathrm{y}, \mathrm{z}$. According to Supplementary Table 4 this results in the vector $\mathbf{r} = (0.70, -0.14, -0.06)$, which represents a physical state. Note that as the Bloch vector is not close to being pure, a simple direct inversion method is sufficient as a tomographic reconstruction method[7]. In Supplementary Figure 2 we compare the measured qubit fidelity with the classical limit proposed by Specht et al.[6].

Supplementary Figure 3 shows the oscilloscope traces collected at readout of a storage experiment of two bright input pulses in adjacent time modes, analogous to the qubit storage. The traces display the transmitted component of the cHSH analyzer pulse followed by the retrieved modes, showing interference in a time bin of 1.65 µs. The interference pattern depends on the cHSH phase $\theta$ and corresponds to the case of two orthogonal projections on the x basis in the qubit experiment. After eliminating the background level and integrating the area in the interference bin, we calculate a visibility of 92 % and a fidelity of 96 %. This further suggests that the fidelity at qubit-level is limited by the noise introduced by the RF pulses, which becomes negligible when we use bright pulses as input. The bright pulse fidelity of 96 % could be due to many small technical limitations, such as phase and amplitude fluctuations in the acouso-optic modulators driving both the input and the transfer modes.


[1] B. Lauritzen et al., "Spectroscopic investigations of $Eu^{3+}$:$Y_2SiO_5$ for quantum memory applications," Phys. Rev. B **85**, 115111 (2012).

[2] P. Jobez et al., "Towards highly multimode optical quantum memory for quantum repeaters," Phys. Rev. A **93**, 032327 (2016).

[3] M. S. Silver, R. I. Joseph, and D. I. Hoult, "Selective spin inversion in nuclear magnetic resonance and coherent optics through an exact solution of the bloch-riccati equation," Phys. Rev. A **31**, 2753–2755 (1985).

[4] M. Tian, T. Chang, K. D. Merkel, and W. Randall, "Reconfiguration of spectral absorption features using a frequency-chirped laser pulse," Appl. Opt. **50**, 6548–6554 (2011).

[5] W. B. Mims, "Phase memory in electron spin echoes, lattice relaxation effects in $CaWO_4$: Er, Ce, Mn," Phys. Rev. **168**, 370 (1968).

[6] H. P. Specht et al., "A single-atom quantum memory," Nature **473**, 190–193 (2011).

[7] R. Schmied, "Quantum state tomography of a single qubit: comparison of methods," J. Mod. Opt. **63**, 1744–1758 (2016).

| $T_s$ (ms) | $\mu_{in}$ | $\mu_{out}$ | $p_N$ | $\eta$ (%) | SNR | $\mu_1$ |
|---|---|---|---|---|---|---|
| 20 | $0.711 \pm 0.006$ | $0.0525 \pm 0.0012$ | $0.0073 \pm 0.0012$ | $7.39 \pm 0.04$ | $7.4 \pm 0.5$ | $0.098 \pm 0.002$ |
| 50 | $1.21 \pm 0.01$ | $0.053 \pm 0.003$ | $0.009 \pm 0.002$ | $4.37 \pm 0.04$ | $5.6 \pm 0.7$ | $0.218 \pm 0.008$ |
| 100 | $1.062 \pm 0.007$ | $0.0276 \pm 0.0012$ | $0.0110 \pm 0.0015$ | $2.60 \pm 0.02$ | $2.5 \pm 0.2$ | $0.445 \pm 0.008$ |

**Supplementary Table 2: Extended table of single photon-level storage.** Relevant quantities averaged over all 6 modes for different spin-wave storage times $T_s$. $\mu_{in}$ = input number of photons; $\mu_{out}$ = retrieved number of photon after storage; $p_N$ = number of noise photons; $\eta$ = storage efficiency; SNR= signal-to-noise ratio; $\mu_1$ = number of photons at input equivalent to SNR=1. All photon numbers are obtained from the detector counts by correcting for the detector efficiency and the path losses from the cryostat output to the detector.

| Mode n. | $\mu_{in}$ | $\mu_{out}$ | $p_N$ | $\eta$ (%) | SNR | $\mu_1$ |
|---|---|---|---|---|---|---|
| 1 | $0.697 \pm 0.015$ | $0.055 \pm 0.003$ | $0.0078 \pm 0.0011$ | $0.0797 \pm 0.0017$ | $7.1 \pm 1.2$ | $0.10 \pm 0.02$ |
| 2 | $0.702 \pm 0.015$ | $0.048 \pm 0.003$ | $0.0078 \pm 0.0011$ | $0.0685 \pm 0.0014$ | $6.2 \pm 1.1$ | $0.11 \pm 0.04$ |
| 3 | $0.707 \pm 0.015$ | $0.055 \pm 0.003$ | $0.0084 \pm 0.0011$ | $0.0781 \pm 0.0016$ | $6.6 \pm 1.1$ | $0.11 \pm 0.03$ |
| 4 | $0.727 \pm 0.015$ | $0.050 \pm 0.003$ | $0.0067 \pm 0.0010$ | $0.0692 \pm 0.0014$ | $7.5 \pm 1.3$ | $0.10 \pm 0.03$ |
| 5 | $0.721 \pm 0.015$ | $0.055 \pm 0.003$ | $0.0078 \pm 0.0011$ | $0.0763 \pm 0.0016$ | $7.1 \pm 1.2$ | $0.10 \pm 0.03$ |
| 6 | $0.712 \pm 0.015$ | $0.051 \pm 0.003$ | $0.0052 \pm 0.0010$ | $0.0714 \pm 0.0015$ | $9.8 \pm 1.9$ | $0.073 \pm 0.018$ |

**Supplementary Table 3: Time mode analysis for 20 ms spin storage.** Quantities as in Supplementary Table 2, obtained separately for each storage mode.

| Basis | $\theta$ | Mode n. | Counts | $V$ |
|---|---|---|---|---|
| x | 0 | 3 | 64 | $0.70 \pm 0.04$ |
| | | 6 | 60 | |
| | $\pi$ | 3 | 25 | |
| | | 6 | 19 | |
| y | $-\pi/2$ | 3 | 48 | $-0.14 \pm 0.07$ |
| | | 6 | 36 | |
| | $\pi/2$ | 3 | 58 | |
| | | 6 | 52 | |
| z | | 2 | 248 | $-0.06 \pm 0.03$ |
| | | 3 | 218 | |
| | | 5 | 197 | |
| | | 6 | 281 | |

**Supplementary Table 4: Qubit storage results.** Raw counts obtained from the qubit storage experiment. Two of the six time modes of the memory were used at each storage attempt to double the acquisition rate. The readout pulse shape and relative cHSH phase $\theta$ define the basis projection after storage. $V$ indicates the average visibility obtained for each basis.

| $T_S$ (ms) | Ref. reps. | Storage reps. | Noise reps. |
|---|---|---|---|
| 20 | 27000 | 51799 | 53449 |
| 50 | 13673 | 15693 | 15693 |
| 100 | 31159 | 43500 | 43500 |

**Supplementary Table 5: Experiment repetitions, single photon level storage.** Number of repetitions of each experiment used to accumulate accurate statistics and errors for the single photon level storage datasets. The number of repetitions is indicated for the acquisition of the reference input signal, the retrieved signal after storage, and the noise background.

| Basis \| phase | Ref. reps. | Storage reps. |
|---|---|---|
| x \| 0 | 222578 | 19862 |
| x \| $\pi$ | 222578 | 39600 |
| y \| $-\pi/2$ | 259576 | 33995 |
| y \| $\pi/2$ | 259576 | 33729 |
| z \| 0 | 277692 | 73076 |

**Supplementary Table 6: Experiment repetitions, 20 ms qubit storage.** Number of repetitions of each experiment used to accumulate accurate statistics and errors for the qubit storage datasets. The number of repetitions is indicated for the acquisition of the reference input signal and the retrieved signal after storage with different projection bases and analyzer phases.
